# Supplementary material for: Extended GFDM Framework: OTFS and GFDM Comparison
Source: arXiv:1808.01161 source file (2018-08-03)
Supplement: Supplementary file 1 [file Additional_text.tex]

The frequency domain representation can be generated form the computation of $N$-\ac{DFT} as
\begin{equation}
	\IndexV{\tilde{\ma{x}}}{n} = \sum\limits_{m = 0}^{M-1}\sum\limits_{k=0}^{K-1} d_{k,m} \dft{g}[<n -kM>_N] e^{-j2\pi\frac{m}{M}n}, \label{eq: Discrete model frequency}
\end{equation}
where  $\dft{\ma{x}} = \mbox{N-DFT}\{x\}$.

the discrete signal representation can be expressed according to \ac{GFDM} equation \eqref{eq: Discrete model}
\begin{equation}
\IndexV{\ma{s}}{l} = \sum\limits_{m=0}^{M_o-1}\sum\limits_{n=0}^{N_o-1}\IndexM{\ma{X}_o^T}{m}{n} g_{\text{tx}}[<l-nM_o>_{(N_oM_o)}]  e^{j2\pi \frac{ml}{M_o}}.
\end{equation}
Here, $g_{\text{tx}}[l] = 1,~0\leq l\leq M_o \mbox{ and } $0$ \mbox{ elsewhere}$. Using \eqref{eq: Time domain model} and noting that $\Z{N_o}{M_o}{g_{tx}} = \ma{1}_{N_o\times M_o}$, i.e. all the entries are equal to $1$, then
\begin{equation}
\V{N_o}{M_o}{\ma{s}} = \ma{X}_o\DFT{M_o}^H, 
\end{equation}
and from \eqref{eq:x_vect gfdm} we get 
\begin{equation}
\ma{s} = \Vect{\{\V{N_o}{M_o}{\ma{s}}\}^T} = \Vect{\DFT{M_o}^H\ma{X}_o^T}.
\end{equation}
In other words,

\begin{equation}
\begin{split}
\{\V{N_o}{M_o}{\ma{s}}\}^T &= \DFT{M_o}^H\ma{X}_o^T\\
&= \DFT{M_o}^H \left(\ma{W}_{\text{tx}}^T\odot \ma{D}_P^T\right)\\
&= \frac{1}{M_oN_o}\DFT{M_o}^H \left(\ma{W}_{\text{tx}}^T\odot \left[ \DFT{M_o} \ma{D_o}^T \DFT{N_o}^H\right]\right),\\
\end{split} \label{eq:OTFS as GFDM}
\end{equation} 
where 
\begin{align}
\V{P}{Q}{\mav{a}}&= \left(\unvec{\mav{a}}{Q}{P} \right)^T,  \label{eq:reshape x}\\
\end{align}

Comparing with \eqref{eq: Time domain model}, we see that \eqref{eq:OTFS as GFDM} represents \ac{GFDM} signal $\ma{x}$ that can be generated as 
\begin{equation}
\ma{x} =  \Vect{\{\V{M_o}{N_o}{\ma{x}}\}^T},~ \ma{s} =  \Vect{\{\V{M_o}{N_o}{\ma{x}}\}}.
\end{equation}
The corresponding \ac{GFDM} parameters are $M = M_o$, $K = N_o$, $\Z{M}{K}{\ma{g}} = \frac{1}{N_o}\ma{W}_{\text{tx}}^T$ and $\ma{D} = \ma{D}_o$.

\subsection{Frequency-domain Matrix representation}
Following the same approach on $\dft{\ma{x}}$ defined in \eqref{eq: Discrete model frequency}, we get
\begin{equation}
\begin{split}
\IndexM{\V{K}{M}{\tilde{\ma{x}}}}{q}{p}
&= \sum_{k=0}^{K-1}\IndexM{\V{K}{M}{\tilde{\ma{g}}}}{<q-k>_K}{p}\sum_{m=0}^{M-1} d_{k,m}  e^{-j2\pi\frac{m}{M} p}. \label{eq:frequency-domain}
\end{split}
\end{equation}
Thereby,
\begin{equation}
\begin{split}
{\V{K}{M}{\tilde{\ma{x}}}} =
\frac{1}{K}\DFT{K}\left(\Zbar{K}{M}{\tilde{\ma{g}}}\odot\left[\DFT{K}^H{\ma{D}\DFT{M}}\right]\right), \label{eq: frequency domain model}
\end{split}
\end{equation}
and 
\begin{equation}
\tilde{\ma{x}} = \Vect{\left(\V{K}{M}{\tilde{\ma{x}}}\right)^T}. \label{eq:xf_gfdm}
\end{equation}
With that we get
\begin{align}
\dft{\ma{A}}
&= \PI{M}{K}\U{M}{K}^H \La^{(\dft{g})}\U{M}{K}\PI{M}{K}^T \U{K}{M}\PI{M}{K}. \label{eq: A-FD}
\end{align}
where 
\begin{align}
\La^{(\dft{g})} &= \diag{\Vect{\Z{M}{K}{\dft{\mav{g}}}}}. \label{eq: D-FD}
\end{align}

\subsection{OTFS in GFDM framework }
Despite of its general representation, it is implicitly considered, as stated in the work related to \ac{OTFS}, e.g. \cite{OTFS_Iterative_raviteja2017low} and \cite{OTFS_implementation_farhang2017low}, that 	$g_{\text{tx}}(t)$ is a rectangular pulse of duration $T_o$ and  $T_o{\Delta f}_o = 1$. Therefore, the discrete signal representation can be expressed according to \ac{GFDM} equation \eqref{eq: Discrete model}
\begin{equation}
\IndexV{\ma{s}}{l} = \sum\limits_{m=0}^{M_o-1}\sum\limits_{n=0}^{N_o-1}\IndexM{\ma{X}_o^T}{m}{n} g_{\text{tx}}[<l-nM_o>_{(N_oM_o)}]  e^{j2\pi \frac{ml}{M_o}}.
\end{equation}
Here, $g_{\text{tx}}[l] = 1,~0\leq l\leq M_o \mbox{ and } $0$ \mbox{ elsewhere}$. Using \eqref{eq: Time domain model} and noting that $\Z{N_o}{M_o}{g_{tx}} = \ma{1}_{N_o\times M_o}$, i.e. all the entries are equal to $1$, then
\begin{equation}
\V{N_o}{M_o}{\ma{s}} = \ma{X}_o\DFT{M_o}^H, 
\end{equation}
and from \eqref{eq:x_vect gfdm} we get 
\begin{equation}
\ma{s} = \Vect{\{\V{N_o}{M_o}{\ma{s}}\}^T} = \Vect{\DFT{M_o}^H\ma{X}_o^T}.
\end{equation}
In other words, the \ac{OTFS} signal can be seen as transmitting precoded \ac{OFDM} symbols of length $M_o$.
Moreover, by replacing $\ma{X}_o$  from \eqref{eq:Xo} and \eqref{eq:DP} we get  
\begin{equation}
\begin{split}
\{\V{N_o}{M_o}{\ma{s}}\}^T &= \DFT{M_o}^H\ma{X}_o^T\\
&= \DFT{M_o}^H \left(\ma{W}_{\text{tx}}^T\odot \ma{D}_P^T\right)\\
&= \frac{1}{M_oN_o}\DFT{M_o}^H \left(\ma{W}_{\text{tx}}^T\odot \left[ \DFT{M_o} \ma{D_o}^T \DFT{N_o}^H\right]\right)\\
&= \V{M_o}{N_o}{\ma{x}}.
\end{split} \label{eq:OTFS as GFDM}
\end{equation}
Comparing with \eqref{eq: Time domain model}, we see that \eqref{eq:OTFS as GFDM} represents \ac{GFDM} signal $\ma{x}$ that can be generated as 
\begin{equation}
\ma{x} =  \Vect{\{\V{M_o}{N_o}{\ma{x}}\}^T},~ \ma{s} =  \Vect{\{\V{M_o}{N_o}{\ma{x}}\}}.
\end{equation}

\subsection{OTFS IN LTV channel}
It has been stated in the original work  \cite{OTFS_arxivmonk2016otfs} that under certain conditions that \ac{OTFS} through an \ac{LTV} channel achieve free \ac{ISI}, and thus we get the receive matrix ignoring the additive noise as
\begin{equation}
\ma{Y} = \ma{H}\odot \ma{X}_o.
\end{equation}
However, this feature is independent of the \ac{OTFS} precoding structure, but it is a result of the chosen transmit and receive pulse shapes used for the precoded symbols. One approach is to insert \ac{CP} per each row of $\V{N_o}{M_o}{\ma{s}}$. Consider a frame of $N_o$ \ac{CP}-\ac{OFDM} symbols such that 
\begin{equation}
s^{(t)}[n] = \sum\limits_{k=0}^{N_o-1}s^{(t)}_k[n-M_s], \label{eq:OFDm frame}
\end{equation}
where $M_s = M_o+N_{\text{cp}}$ is the \ac{OFDM} symbol duration and $s^{(t)}_k[n] = s_k[<q-N_{cp}>_{M_o}]$ , $n=0\cdots M_s-1$ with 
\begin{equation}
s_k[n] = \frac{1}{M_o}\sum\limits_{m=0}^{M_o-1}\IndexM{\ma{X}_o}{k}{m}e^{j2\pi\frac{nm}{M_o}}. \label{eq:OFDm symbol}
\end{equation}
The received signal through \ac{LTV} channel $h(\nu, l)$, where $l$ is the delay index and $\nu$ is the normalized Doppler frequency, is given by
\begin{equation}
\begin{split}
s^{(r)}[n] = \int_{\nu} \sum_{l=0}^{L-1}h(l,\nu) s^{(t)}[n-l]e^{j2\pi n\nu}d\nu,
\end{split}
\end{equation}
with $L\leq N_{\text{cp}}-1$ is the maximum delay.
Then we extract the samples $Y[n,m]$ as
\begin{equation}
\begin{split}
Y[k, p] &= s^{(r)}[N_{cp} + p+ kM_s],~ m=0\cdots M_o-1, k = 0,\cdots N_o-1\\
&= \int_{\nu} \sum_{l=0}^{L-1}h(l,\nu) s_k[<p-l>_{M_o}]e^{j2\pi [N_{cp} + p+ kM_s]\nu}d\nu\\
&=\int_{\nu} \frac{1}{M_o}\sum_{m=0}^{M_o-1}\tilde{h}(m,\nu) \IndexM{\ma{X}_o}{k}{m}e^{j2\pi\frac{mp}{M_o}}e^{j2\pi [N_{cp} + p+ kM_s]\nu}d\nu.
\end{split}
\end{equation}
This corresponds to removing the \ac{CP} from each symbol and the convolution with the channel becomes circular due to the \ac{CP} insertion.
Then we apply $M_o$-\ac{DFT} per \ac{OFDM} symbols, therefore, 

\begin{equation}
\begin{split}
\bar{Y}[k, u] &=\sum_{p=0}^{M_o-1}Y[k, p]e^{-j2\pi\frac{pu}{M_o}}\\
& =\int_{\nu} \left(
\begin{array}{c}
\frac{1}{M_o}\sum\limits_{m=0}^{M_o-1}\tilde{h}(m,\nu) \IndexM{\ma{X}_o}{k}{m} e^{j2\pi [N_{cp}+ kM_s]\nu}\\
\cdot \sum\limits_{p=0}^{M_o-1}e^{j2\pi\frac{p(m-u)}{M_o}}e^{j2\pi p\nu}
\end{array}
\right) d\nu.
\end{split}
\end{equation}
Assume the maximum Doppler spread $|f_D| \ll \frac{1}{M_o}$ then we get
\begin{equation}
\sum\limits_{p=0}^{M_o-1}e^{j2\pi\frac{p(m-u+\nu)}{M_o}} \approx \sum\limits_{p=0}^{M_o-1}e^{j2\pi p\nu}\delta(m-u)
\end{equation}
as a result 

\begin{equation}
\begin{split}
\bar{Y}[k, u] &=\sum_{p=0}^{M_o-1}Y[q, p]e^{-j2\pi\frac{pu}{M_o}}\\
& =\IndexM{\ma{X}_o}{k}{u}\frac{1}{M_o}\sum\limits_{p=0}^{M_o-1} \int_{\nu} 
\tilde{h}(u,\nu)  e^{j2\pi [N_{cp}+ kM_s +p]\nu}
d\nu\\
&= \IndexM{\ma{X}_o}{k}{u}\frac{1}{M_o}\sum\limits_{p=0}^{M_o-1} 
\tilde{H}(u,N_{cp}+ kM_s +p)  
\end{split}
\end{equation}
where $\tilde{H}(n, u) $ is the channel response in time-frequency domain. 
Actually, the \ac{CP} eliminate the \ac{ISI} between the \ac{OFDM} symbols, and due to larger subcarrier spacing, then the \ac{ISI} within one \ac{OFDM} is 	
neglected. The problem is that the overhead due to \ac{CP} is very high, however, the spreading might be useful for diversity. Consider no windowing, then 
\begin{equation}
\ma{Y} = \frac{1}{M_o N_o}\ma{H}\odot \left[ \DFT{N_o}^H\ma{D}_o\DFT{M_o} \right]
\end{equation}

Actually, this permutation of the data symbols affects the spectral properties of the waveform.

\begin{equation}
\begin{split}
\bar{Y}[k, u] &=\sum_{p=0}^{M_o-1}Y[q, p]e^{-j2\pi\frac{pu}{M_o}}\\
& =\IndexM{\ma{X}_o}{k}{u}\sum\limits_{p=0}^{M_o-1} \int_{\nu} 
\tilde{h}(u,\nu)  e^{j2\pi [N_{cp}+ kM_s +p]\nu}
d\nu\\
&= \IndexM{\ma{X}_o}{k}{u}\sum\limits_{p=0}^{M_o-1} 
\tilde{H}(u,N_{cp}+ kM_s +p)  
\end{split}
\end{equation}

\subsection{OTFS in frequency domain}
Consider that $\tilde{\ma{g}}_{\text{tx}}$ is rectangular in frequency then 
using \eqref{eq: frequency domain model} of \ac{GFDM} so that 
\begin{equation}
\V{M_o}{N_o}{\tilde{\ma{s}}} = \ma{X}_0^T\DFT{N_o}.
\end{equation}

\begin{equation}
\tilde{\ma{s}} = \Vect{\{\V{M_0}{N_0}{\tilde{\ma{s}}}\}^T} = \Vect{\DFT{N_o}\ma{X}_0}.
\end{equation}
Moreover, by replacing $\ma{X}_0$  from \eqref{eq:Xo} and \eqref{eq:DP} we  
\begin{equation}
\begin{split}
\{\V{M_0}{N_0}{\tilde{\ma{s}}}\}^T &= \DFT{N_0}\ma{X}_0\\
&= \DFT{N_0} \left(\ma{W}_{\text{tx}}\odot \ma{D}_P\right)\\
&= \frac{1}{M_oN_o}\DFT{N_0} \left(\ma{W}_{\text{tx}}\odot \left[ \DFT{N_o}^H \ma{D_o} \DFT{M_o}\right]\right)\\
&= \V{N_0}{M_0}{\tilde{\ma{x}}}.
\end{split} 
\end{equation}
The corresponding \ac{GFDM} parameters are $M = M_o$, $K = N_0$, $\Z{M}{K}{\ma{g}} = \frac{1}{N_0}\ma{W}_{\text{tx}}^T$ and $\ma{D} = \ma{D}_o$. The essential difference to the \ac{GFDM} is the transpose operation at the final step, as depicted in 

\section{Appendix}\label{sec:append}
Consider a \ac{LTV}  in the continuous model representation $h_c(t,\tau)$ with Doppler-delay $H_c(\nu, \tau)$ and a transmitted signal $s(t)$,  the received signal can be written as 
\begin{equation}
\begin{split}
r(t) &= \int  h_c(t, \tau) s(t-\tau)d\tau \\
& = 
\int \int H_c(\nu, \tau) s(t-\tau)e^{j2\pi\nu t}d\tau d\nu\\
\end{split}
\end{equation}

For a discrete
\begin{equation}
s(t) = \sum_{q} s[q] \delta(t-qT_s),
\end{equation}
where $F_s = \frac{1}{T_s}$ is the sampling frequency, then
\begin{equation}
\begin{split}
r[t] &= \int_{\nu} \int_{\tau} H_c[\nu, t-\tau]  \sum_{q}s[q] \delta(\tau-qT_s) e^{j2\pi t\nu}\\
&= \int_{\nu} \sum_{q} s[q] H_c(\nu, t-qT_s) e^{j2\pi t\nu}d\tau d\nu. 
\end{split}
\end{equation}
By sampling the received signal we get, 
\begin{equation}
r[n] = \int_{\nu} \sum_{q} s[q] H_c(\nu, nT_s-qT_s)   e^{j2\pi \frac{n\nu}{F_s}} d\nu 
\end{equation}
the equivalent discrete channel can be written as 
\begin{equation}
H(\nu, q)= H_c(\nu, qT_s). 
\end{equation}
Therefore,
\begin{equation}
\begin{split}
r[n] &= \int_{\nu} \left[ \sum_{q} H(\nu, n-q) s[q]\right]    e^{j2\pi \frac{n\nu}{F_s}}d\nu\\
&= \int_{\nu} S(\nu, n)  e^{j2\pi \frac{n\nu}{F_s}}d\nu.
\end{split}
\end{equation}
Here, 
\begin{equation}
S(\nu, n) = \sum_{q} H(\nu, n-q) s[q].
\end{equation}
for a maximum delay spread $\tau_{\text{max}}$ the discrete channel can be modeled as \ac{FIR} filter with $L$ taps. In addition, the  maximum Doppler spread  $f_D$ can be defined, such that $H(\nu, q)  = 0, ~ \nu> |f_D/2|$.

In relation to subcarrier spacing, the normalized Doppler frequency can be normalized to the subcarrier spacing, such that $f_d = \frac{\nu}{\Delta f}$, and then with $F_s = B = K\Delta f$. We finally get, 

\begin{equation}
\begin{split}
r[n]&= \Delta f\int\limits_{-\tfrac{f_D}{2\Delta f}}^{\tfrac{f_D}{2\Delta f}} S(f_d\Delta f, n)  e^{j2\pi \frac{nf_d}{K}}d f_d.
\end{split}
\end{equation}
We can select the subcarrier spacing to satisfy $\frac{fD}{\Delta f}\leq 1$, then 

\begin{equation}
\begin{split}
r[n]&= \int\limits_{-1/2}^{1/2} S(f_d, n)  e^{j2\pi \frac{nf_d}{K}}d f_d.
\end{split}
\end{equation}
This integration can be approximated by  sum  with step $\frac{1}{M}$ such that
\begin{equation}
\begin{split}
r[n]&= \sum\limits_{m = -M/2}^{M/2} S\left(\tfrac{m}{M}, n\right)  e^{j2\pi \frac{nm}{MK}} \tfrac{1}{M}.
\end{split}
\end{equation}

Further simplification. 
\begin{equation}
\begin{split}
r[n]&=\tfrac{1}{M} \sum\limits_{m = 0}^{M-1} S\left(m, n\right)  e^{j2\pi \frac{nm}{MK}}.
\end{split}
\end{equation}

Therefore, the time invariant channel can be equivalently represented by 
\begin{equation}
\begin{split}
r[n]&=\sum\limits_{m = 0}^{M-1} S\left(m, n\right)  e^{j2\pi \frac{nm}{MK}}\\
&= \tfrac{1}{M} \sum\limits_{m = 0}^{M-1}\sum\limits_{l=0}^{L-1} H[m, n-l] s[l] e^{j2\pi \frac{nm}{MK}}
\end{split}
\end{equation}
Thus, the final channel model can be seen as time variant \ac{FIR} with gain defined by the function $H[m,l]$ and Doppler shift $\frac{m}{N}$, $N = MK$.

Consider a short burst of duration $N$ and a \ac{CP} of length  $N_{\text{cp}}\geq L-1$, is added to a signal $x[n]$ such that,
so that $s[n] = x[<n-N_{cp}>_N]$, $N_s = N+N_{\text{cp}}$
\begin{equation}
\begin{split}
y_i[n]&=r[n+N_{cp} + i(N+N_{\text{cp}})], ~ n = 0\cdots, N-1\\
&= \sum\limits_{m = 0}^{M-1}\sum\limits_{l=0}^{L-1} H[m, l] x[<n-l>_N] e^{j2\pi \frac{(n+(i+1)N_{cp})m}{MK}}\\
&= \sum\limits_{m = 0}^{M-1}\sum\limits_{q=0}^{N-1} \tilde{H}[m, q] \tilde{x}[q] e^{j2\pi \frac{(n+[i+1]N_{\text{cp}})m}{MK}}e^{j2\pi\frac{nq}{N}}\\	
&=\sum\limits_{m = 0}^{M-1} e^{j2\pi \frac{(n+[i+1]N_{\text{cp}})m}{MK}} \sum\limits_{q=0}^{N-1} \tilde{H}[m, q] \tilde{x}[q]e^{j2\pi\frac{nq}{N}}\\
&=\sum\limits_{m = 0}^{M-1} e^{j2\pi \frac{[i+1]N_{\text{cp}}m}{MK}}
\IndexM{\DFT{N}^H}{n}{m}
\IndexV{\DFT{N}^H\left[\tilde{\ma{h}}_m\odot \tilde{\ma{x}}_i\right]}{n}\\
&=  \ma{H}^{(eq)}_i\tilde{\ma{x}}_i
\end{split}
\end{equation}

\begin{equation}
\begin{split}
\ma{H}^{(eq)}_i &= \sum\limits_{m = 0}^{M-1} e^{j2\pi \frac{[i+1]N_{\text{cp}}m}{MK}}
\ma{\Lambda}_m
\DFT{N}^H \ma{\Lambda}^{\ma{\tilde{h}}}_m
\end{split}
\end{equation}

\begin{equation}
\begin{split}
\IndexM{\ma{H}^{(eq)}_i}{q}{p} &= \sum\limits_{m = 0}^{M-1} e^{j2\pi \frac{[i+1]N_{\text{cp}}m}{MK}}
e^{j2\pi\frac{qm}{N}}e^{j2\pi\frac{qp}{N}}\IndexM{\tilde{\ma{H}}^{(ch)}}{m}{p}\\
&= e^{j2\pi\frac{qp}{N}}\sum\limits_{m = 0}^{M-1} e^{j2\pi \frac{[i+1]N_{\text{cp}}m}{MK}}
e^{j2\pi\frac{qm}{N}}\IndexM{\tilde{\ma{H}}^{(D-F)}}{m}{p}\\
&=\DFT{N}^H\odot \ma{H}^{(T-F)}
\end{split}
\end{equation}

\begin{equation}
\begin{split}
\IndexM{\tilde{\ma{H}}^{(eq)}_i}{q}{p} =  \sum\limits_{n=0}^{N-1} e^{-2j\pi\frac{qn}{N}}\IndexM{{\ma{H}}^{(eq)}_i}{n}{p} e^{-2j\pi\frac{np}{N}}
\end{split}
\end{equation}
\begin{equation}
\begin{split}
\ma{y}_i &= \sum\limits_{m = 0}^{M-1} e^{j2\pi \frac{[i+1]N_{\text{cp}}m}{MK}}
\IndexM{\DFT{N}^H}{:}{m}
\odot \IndexV{\DFT{N}^H\left[\tilde{\ma{h}}_m\odot \tilde{\ma{x}}_i\right]}{n}
\end{split}
\end{equation}

Let $\ma{H}_m \in \compl^{N\times N}$ be the corresponding circular channel matrix generated from the vector $\ma{h}_m \in \compl^{N\times 1}$, where 
\begin{equation}
\IndexV{\ma{h}_m}{l} = H[m,l], ~0<l<L-1 \mbox{ and $0$ elsewhere}
\end{equation}
then we get 
\begin{equation}
\begin{split}
\ma{y}_i &= \sum\limits_{m = 0}^{M-1} e^{j2\pi \frac{[i+1]N_{\text{cp}}m}{N}} \diag{\IndexM{\DFT{N}^H}{:}{m}}\ma{H}_m\ma{x}_i\\
&= \ma{H}^{(eq)}_i\tilde{\ma{x}}_i
\end{split}
\end{equation}
\begin{equation}
\ma{H}^{(eq)}_i = \sum\limits_{m = 0}^{M-1} e^{j2\pi \frac{[i+1]N_{\text{cp}}m}{N}} \diag{\IndexM{\DFT{N}^H}{:}{m}}\DFT{N}^H\diag{\tilde{\ma{h}}_m}
\end{equation}
Thus
\begin{equation}
\begin{split}
\IndexM{\ma{\ma{H}^{(eq)}_i}}{q}{p} &= \sum\limits_{m = 0}^{M-1}e^{j2\pi \frac{[i+1]N_{\text{cp}}m}{N}}e^{j2\pi\frac{qp}{N}} e^{j2\pi\frac{qm}{N}} \IndexM{\tilde{\ma{H}}}{m}{p}\\
&=e^{j2\pi\frac{qp}{N}} \sum\limits_{m = 0}^{M-1}e^{j2\pi \frac{[i+1]N_{\text{cp}}m}{N}} e^{j2\pi\frac{qm}{N}} \IndexM{\tilde{\ma{H}}}{m}{p}
\end{split}
\end{equation}
In addition let if $H(\nu, l) = 0$, $|\nu| > F_D/2$
In this case
\begin{equation}
\begin{split}
h_i[n,l] & = h[n+N_{cp}+iN_s,l]~ , ~n = 0\cdots N-1\\
&= \int_{\nu}h(\nu, l) e^{j2\pi\frac{\nu}{F_s}(n+N_{cp}+iN_s)}\\
\end{split} d\nu 
\end{equation}
by computing $N$-DFT we get 

\begin{equation}
\begin{split}
\tilde{h}_i[q,l] &= \sum_{n=0}^{N-1}\int_{\nu}h(\nu, l) e^{j2\pi\frac{\nu}{F_s}(n+N_{cp}+iN_s)}e^{-j2\pi\frac
	{qn}{N}} d\nu \\
&= \int\limits_{\nu = -F_D/2}^{\nu = F_D/2} e^{j2\pi\frac{\nu}{F_s}(N_{cp}+iN_s)}h(\nu, l)\sum_{n=0}^{N-1} e^{j2\pi\frac{\nu}{F_s}n}e^{-j2\pi\frac
	{qn}{N}} d\nu \\
&= \int\limits_{\nu = -F_D/2}^{\nu = F_D/2} e^{j2\pi\frac{\nu}{F_s}(N_{cp}+iN_s)}h(\nu, l) e^{j\pi[\tfrac{\nu}{F_s} - f](N-1)} \frac{\sin(\pi[N\tfrac{\nu}{F_s} - q])}{\sin(\pi[\tfrac{\nu}{F_s} - f])}
\end{split}
\end{equation}
$N$ can be chosen such that $N\tfrac{F_D}{F_s} \leq 1 $ and thus $\tilde{h}_i[q,l]$ is non zero for $ q_{\text{min}}\leq q\leq q_{\text{max}}$. so the discrete Doppler domain has finite taps of length $Q$, and thus we can write
\begin{equation}
y_i[n] = \sum_{q=0}^{Q-1}\sum_{l=0}^{L-1} \tilde{h}_i[q,l] x_i[<n-l>_N] e^{j2\pi\frac{qn}{N}}
\end{equation}

Let $L\leq K$ and $Q\leq M$, then

Let define
\begin{equation}
X^{(cp)}[m,k] = x[<m+(k-K_{\text{cp}})M>_K]
\end{equation}
and 
\begin{equation}
s = \Vect{X^{(cp)}}
\end{equation}

\begin{equation}
\begin{split}
r[n]&= \sum\limits_{l=0}^{L-1} h[n,l] s[n-l]  
\end{split}
\end{equation}
\begin{equation}
\begin{split}
Y[m,k] &=r[m+k(M+M_{cp}) + M_{\text{cp}}] \\
& = \sum\limits_{l=0}^{L-1} h[m+k(M+M_{cp},l] s[m+k(M+M_{cp}) + M_{\text{cp}}-l]\\
&= \sum\limits_{l=0}^{L-1} h[m+k(M+M_{cp}),l] X[m-l,k]\\
&=\sum\limits_{l=0}^{L-1} h_k[m,l] X[m-l,k]\\
\tilde{Y}[p,k]&= \sum_{l=0}^{M-1} h_k[,f]\tilde{X}[f,k] e^{j2\pi\frac{pm}{M}}
\end{split} 
\end{equation}

\section{LTV}
\onecolumn
The transmitted signal 
\begin{equation}
x[n] = \sum\limits_{k=0}^{K-1}\sum\limits_{m=0}^{M-1} d_{k,m}g_{k,m}^{(t)}[n]
\end{equation}
The received signal through \ac{LTV} 
\begin{equation}
r[n] = \int_{\nu}\sum\limits_{l=0}^{L-1} H[l, \nu] x[n-l]e^{j2\pi n\nu } d\nu
\end{equation}
applying a received pulse $g^{(rx)}[n]$ we get
\begin{equation}
\begin{split}
R^{(y)}[p, f] &= \sum_{n} g^{*(rx)}[n-p]r[n] e^{-j2\pi n f }\\
&= \int_{\nu}\sum\limits_{l=0}^{L-1} H[l, \nu] \sum_{n} g^{*(rx)}[n-p] e^{-j2\pi nf} x[n-l]e^{j2\pi n \nu} d\nu\\
& = \int_{\nu}\sum\limits_{l=0}^{L-1} H[l, \nu] R^{(x)}[p-l,f-\nu ] e^{-j2\pi(f-\nu)l}d\nu
\end{split}
\end{equation}

\begin{equation}
\begin{split}
R^{(x)}[p,f] & = \sum_{n} g^{*(rx)}[n-p]x[n] e^{-j2\pi nf}\\
&= \sum\limits_{\bar{k}=0}^{K-1}\sum\limits_{\bar{m}=0}^{M-1} d_{\bar{k},\bar{m}} \sum_{n} g^{*(rx)}[n-p]g_{\bar{k},\bar{m}}^{(tx)}[n]e^{-j2\pi nf}\\
&= \sum\limits_{\bar{k}=0}^{K-1}\sum\limits_{\bar{m}=0}^{M-1} d_{\bar{k},\bar{m}} R^{(g^{(tx)}_{\bar{k},\bar{m}})}[p,f]
\end{split}
\end{equation}

\begin{equation}
\begin{split}
R^{(y)}[p, f] = 
&\sum\limits_{\bar{k}=0}^{K-1}\sum\limits_{\bar{m}=0}^{M-1} d_{\bar{k},\bar{m}}  \int_{\nu}\sum\limits_{l=0}^{L-1} H[l, \nu] R^{(g^{(tx)}_{\bar{k},\bar{m}})}[p-l,f-\nu ] e^{-j2\pi(f-\nu)l}d\nu
\end{split}
\end{equation}
The estimated data symbol can be computed by sampling $R^{(y)}[p, q]$ at points $(p_m, q_k)$ to get  $d_{m,k}$ such that
\begin{equation}
\hat{d}_{k,m} = R^{(y)}_{k,m}[p_m, f_k ]
\end{equation}
In order to get free interference we need to satisfy the condition 
\begin{equation}
A(k,m,\bar{k},\bar{m}) = \int_{\nu}\sum\limits_{l=0}^{L-1} H[l, \nu] R^{(g^{(tx)}_{\bar{k},\bar{m}})}[p_m-l,f_k-\nu ] e^{-j2\pi(f_k-\nu)l}d\nu = C_{k,m} \delta(m-\bar{m})\delta(k-\bar{k})
\end{equation}

\begin{equation}
\begin{split}
R^{(g^{(tx)}_{\bar{k},\bar{m}})}[p,f ] = \sum_{n} g^{*(rx)}[n-p]g_{\bar{k},\bar{m}}^{(tx)}[n]e^{-j2\pi fn}
\end{split}
\end{equation}

\begin{equation}
\begin{split}
A(k,m,\bar{k},\bar{m}) &= \int_{\nu}\sum\limits_{l=0}^{L-1} H[l, \nu] e^{-j2\pi f_kl}\sum_{n} g^{*(rx)}[n+l-p_m]g_{\bar{k},\bar{m}}^{(tx)}[n]e^{-j2\pi f_kn} e^{j2\pi (n+l)\nu} d\nu\\
&= \int_{\nu}\sum\limits_{l=0}^{L-1} H[l, \nu] e^{-j2\pi f_kl}C(k,m,\bar{k},\bar{m}, l , \nu) d\nu
\end{split}
\end{equation}
\subsection{Circuilar design}

\begin{equation}
g_{\bar{k},\bar{m}}^{(tx)}[n] = g_{\bar{m},\bar{k}}[<n-N_{\text{cp}}>_N],~  0\cdots N+N_{cp}-1
\end{equation}
with 
\begin{equation}
g_{\bar{m},\bar{k}}[n] = g[<n-\bar{m}K>_N]e^{j2\pi\frac{\bar{k}}{K}n}
\end{equation}
where 
$g[n] = 1,~ n=0\cdots K+N_{cp}$
and the receiver pulse shape is rectangular and periodic  
\begin{equation}
g^{*(rx)}[n] =\left\lbrace \begin{array}{cc}
0&, n=0\cdots N_{cp}-1\\
1&, n = N_{cp}\cdots N+N_{cp}-1\\
0& \mbox{elsewhere}
\end{array} \right\rbrace
\end{equation}
Let $f_k = \frac{k}{K}$, $p_m = mK $. 

\begin{equation}
\begin{split}
C(k,m,\bar{k},\bar{m}, l , \nu) &= \sum_{n} g^{*(rx)}[n+l-mK ]g^{(tx)}_{\bar{k},\bar{m}}[n]  e^{-j2\pi \tfrac{k}{K}n} e^{j2\pi (n+l)\nu}\\
&= \sum_{n} g^{*(rx)}[n]g^{(tx)}_{\bar{k},\bar{m}}[n-l+mK]  e^{-j2\pi \tfrac{k}{K}(n-l)} e^{j2\pi (n+mK)\nu}\\
&=\sum\limits_{n=N_{cp}}^ {N+N_{cp}-1}g^{(tx)}_{\bar{k},\bar{m}}[n-l+mK]  e^{-j2\pi \tfrac{k}{K}(n-l)} e^{j2\pi (n+mK)\nu}\\
&=\sum\limits_{n=0}^ {N-1}g^{(tx)}_{\bar{k},\bar{m}}[n-l+mK+N_{cp}]  e^{-j2\pi \tfrac{k}{K}(n-l+N_{cp})} e^{j2\pi (n+mK+N_{cp})\nu}\\
&=  e^{j2\pi (mK+N_{cp})\nu}e^{-j2\pi \tfrac{k}{K}(N_{cp})} e^{j2\pi l\nu} \sum\limits_{n=0}^ {N-1}g[<n-l-(\bar{m}-m)K>_N] e^{-j2\pi \tfrac{k-\bar{k}}{K}(n-l)}  e^{j2\pi (n-l)\nu}\\
&= 
\end{split}
\end{equation}
If $g[n] = 1, n=0\cdots, K-1$, which is equivalent to transmitting successive OFDM with one CP, then 

\begin{equation}
\begin{split}
C(k,m,\bar{k},\bar{m}, l , \nu) &= e^{j2\pi (mK+N_{cp})\nu}e^{-j2\pi \tfrac{k}{K}(N_{cp})} e^{j2\pi l\nu} \sum\limits_{n=l+(\bar{m}-m)K}^{l+(\bar{m}-m)K + K-1} e^{-j2\pi \tfrac{k-\bar{k}}{K}(n-l)}  e^{j2\pi (n-l)\nu}\\
&=e^{j2\pi (\bar{m}K+N_{cp})\nu}e^{-j2\pi \tfrac{k}{K}(N_{cp})} e^{j2\pi l\nu} \sum\limits_{n=0}^{K-1} e^{-j2\pi \tfrac{k-\bar{k}}{K}n}  e^{j2\pi n\nu}\\
& \approx e^{j2\pi (\bar{m}K+N_{cp})\nu}e^{-j2\pi \tfrac{k}{K}(N_{cp})} e^{j2\pi l\nu} \sum\limits_{n=0}^{K-1} e^{j2\pi n\nu} \delta(\bar{k}-k)
\end{split}
\end{equation}
If Doppler shift is small 

\begin{equation}
\begin{split}
A(k,m,\bar{k},\bar{m}) &= \int_{\nu}\sum\limits_{l=0}^{L-1} H[l, \nu] e^{-j2\pi f_kl}\sum_{n} g^{*(rx)}[n+l-p_m]g_{\bar{k},\bar{m}}^{(tx)}[n]e^{-j2\pi f_kn} e^{j2\pi (n+l)\nu} d\nu\\
&= \int_{\nu}\sum\limits_{l=0}^{L-1} H[l, \nu] e^{-j2\pi \frac{kl}{K}}e^{j2\pi (\bar{m}K+N_{cp})\nu}e^{-j2\pi \tfrac{k}{K}(N_{cp})} e^{j2\pi l\nu} \sum\limits_{n=0}^{K-1} e^{j2\pi n\nu} \delta(\bar{k}-k) d\nu
\end{split}
\end{equation}

\begin{equation}
\begin{split}
&=e^{-j2\pi\frac{N_{\text{cp}}\bar{k}}{K}} \sum_{n} g^{*(rx)}[n+l-m(N_{cp}+K)]g[n-\bar{m}(K+N_{\text{cp}})] e^{j2\pi \frac{\bar{k}-k}{K}n} e^{j2\pi (n+l)\nu}\\
&= e^{-j2\pi\phi[k,m,\bar{k} , \nu]}\sum\limits_{n = N_{cp}-l}^{K+N_{cp}-l-1} e^{j2\pi \frac{\bar{k}-k}{K}n} e^{j2\pi (n+l)\nu}\delta(m-\bar{m})\\
&= e^{-j2\pi\phi[k,m,\bar{k} , \nu]}\sum\limits_{n = 0}^{K-1} e^{j2\pi \frac{\bar{k}-k}{K}(n+N_{cp}-l)} e^{j2\pi (n+N_{cp})\nu}\delta(m-\bar{m})\\
&=  e^{j2\pi\phi[k,m,\bar{k} , \nu]}e^{j2\pi \frac{\bar{k}-k}{K}(N_{cp}-l)} e^{j2\pi N_{cp}\nu} \sum\limits_{n = 0}^{K-1} e^{j2\pi \frac{\bar{k}-k}{K}n} e^{j2\pi n\nu}\delta(m-\bar{m})\\
&=e^{j2\pi \tfrac{N_{cp}(m+1)[\bar{k}-k] - N_{cp}\bar{k}}{K}}e^{-j2\pi\frac{l[\bar{k}-k] }{K}}e^{j2\pi[N_{cp}(m+1)\nu + mK\nu]} \sum\limits_{n = 0}^{K-1} e^{j2\pi \frac{\bar{k}-k}{K}n} e^{j2\pi n\nu}\delta(m-\bar{m})\\
& =e^{j2\pi \tfrac{N_{cp}(m+1)[\bar{k}-k] - N_{cp}\bar{k}}{K}}e^{-j2\pi\frac{l[\bar{k}-k] }{K}}e^{j2\pi[N_{cp}(m+1)\nu + mK\nu]}  e^{j2\pi [K\nu +\bar{k}-k]\frac{K-1}{K}}\frac{\sin(\pi[\bar{k}-k + K\nu])}{\sin(\pi\tfrac{[\bar{k}-k + K\nu]}{K})}\delta(m-\bar{m})
\end{split}
\end{equation}

\subsection{Design}
The CP-\ac{OFDM} approach 
\begin{equation}
g_{\bar{k},\bar{m}}^{(tx)}[n] = g[n-\bar{m}(K-N_{\text{cp}})] e^{j2\pi\frac{(n-N_{\text{cp}})\bar{k}}{K}}
\end{equation}
where 
$g[n] = 1,~ n=0\cdots K+N_{cp}$
and 
\begin{equation}
g^{*(rx)}[n] =\left\lbrace \begin{array}{cc}
0&, n=0\cdots N_{cp}-1\\
1&, n = N_{cp}\cdots K+N_{cp}-1\\
0& \mbox{elsewhere}
\end{array} \right\rbrace
\end{equation}
This design is equivalent to remove CP.
Let $p_m = N_{cp}+m(N_{cp}+K)$, $q_k = \tfrac{k}{K}$
\begin{equation}
\begin{split}
C(k,m,\bar{k},\bar{m}, l , \nu) &= \sum_{n} g^{*(rx)}[n+l-m(N_{cp}+K)]g[n-\bar{m}(K+N_{\text{cp}})] e^{j2\pi\frac{(n-N_{\text{cp}})\bar{k}}{K}} e^{-j2\pi \tfrac{k}{K}n} e^{j2\pi (n+l)\nu}\\
&=e^{-j2\pi\frac{N_{\text{cp}}\bar{k}}{K}} \sum_{n} g^{*(rx)}[n+l-m(N_{cp}+K)]g[n-\bar{m}(K+N_{\text{cp}})] e^{j2\pi \frac{\bar{k}-k}{K}n} e^{j2\pi (n+l)\nu}\\
&=  e^{-j2\pi \phi[k,m,\bar{k} , \nu]}\sum_{n} g^{*(rx)}[n+l]g[n-(\bar{m}-m)(K+N_{\text{cp}})] e^{-j2\pi \frac{\bar{k}-k}{K}n} e^{j2\pi (n+l)\nu}\\
&= e^{-j2\pi\phi[k,m,\bar{k} , \nu]}\sum\limits_{n = N_{cp}-l}^{K+N_{cp}-l-1} e^{j2\pi \frac{\bar{k}-k}{K}n} e^{j2\pi (n+l)\nu}\delta(m-\bar{m})\\
&= e^{-j2\pi\phi[k,m,\bar{k} , \nu]}\sum\limits_{n = 0}^{K-1} e^{j2\pi \frac{\bar{k}-k}{K}(n+N_{cp}-l)} e^{j2\pi (n+N_{cp})\nu}\delta(m-\bar{m})\\
&=  e^{j2\pi\phi[k,m,\bar{k} , \nu]}e^{j2\pi \frac{\bar{k}-k}{K}(N_{cp}-l)} e^{j2\pi N_{cp}\nu} \sum\limits_{n = 0}^{K-1} e^{j2\pi \frac{\bar{k}-k}{K}n} e^{j2\pi n\nu}\delta(m-\bar{m})\\
&=e^{j2\pi \tfrac{N_{cp}(m+1)[\bar{k}-k] - N_{cp}\bar{k}}{K}}e^{-j2\pi\frac{l[\bar{k}-k] }{K}}e^{j2\pi[N_{cp}(m+1)\nu + mK\nu]} \sum\limits_{n = 0}^{K-1} e^{j2\pi \frac{\bar{k}-k}{K}n} e^{j2\pi n\nu}\delta(m-\bar{m})\\
& =e^{j2\pi \tfrac{N_{cp}(m+1)[\bar{k}-k] - N_{cp}\bar{k}}{K}}e^{-j2\pi\frac{l[\bar{k}-k] }{K}}e^{j2\pi[N_{cp}(m+1)\nu + mK\nu]}  e^{j2\pi [K\nu +\bar{k}-k]\frac{K-1}{K}}\frac{\sin(\pi[\bar{k}-k + K\nu])}{\sin(\pi\tfrac{[\bar{k}-k + K\nu]}{K})}\delta(m-\bar{m})
\end{split}
\end{equation}
Putting all together
\begin{equation}
\begin{split}
C(k,m,\bar{k},\bar{m}, l , \nu)
&=e^{-j2\pi\phi_0(\bar{k}, k, m, N_{cp})}e^{-j2\pi\phi(l,\nu)} C(\bar{k}-\bar{k}, \nu) \delta(m-\bar{m})
\end{split}
\end{equation}

if the maximum Doppler spread is significantly smaller than the subcarrier spacing, i.e. $|\nu|\ll \frac{1}{K}$
then 
\begin{equation}
\frac{\sin(\pi[\bar{k}-k + K\nu])}{\sin(\pi\tfrac{[\bar{k}-k + K\nu]}{K})}\approx \frac{\sin(\pi  K\nu)}{\sin(\pi \nu)} \delta(\bar{k}-k)
\end{equation}
then 
\begin{equation}
\begin{split}
C(k,m,\bar{k},\bar{m}, l , \nu) & = e^{-j2\pi \frac{N_{cp}\bar{k}}{K}}e^{j2\pi[N_{cp}(m+1)\nu + K\nu]} \sum\limits_{n = 0}^{K-1}  e^{j2\pi n\nu}\delta(m-\bar{m})\delta(k-\bar{k})\\	
\end{split}
\end{equation}
\begin{equation}
\begin{split}
A(k,m,\bar{k},\bar{m}) 
&= e^{-j2\pi \frac{N_{cp}\bar{k}}{K}}\sum\limits_{n = 0}^{K-1}\int_{\nu}\sum\limits_{l=0}^{L-1} H[l, \nu] e^{-j2\pi[N_{cp}(m+1)\nu + K\nu]} e^{-j2\pi\tfrac{k}{K}l}  e^{j2\pi n\nu}\delta(m-\bar{m})\delta(k-\bar{k}) d\nu\\
&=  e^{-j2\pi \frac{N_{cp}\bar{k}}{K}}\sum\limits_{n = 0}^{K-1}\int_{\nu} \tilde{H}[k, \nu] e^{j2\pi[N_{cp}(m+1)\nu + mK\nu]}  e^{j2\pi n\nu}\delta(m-\bar{m})\delta(k-\bar{k}) d\nu\\
&=e^{-j2\pi \frac{N_{cp}{k}}{K}}\sum\limits_{n = 0}^{K-1} \bar{\tilde{H}}[k, n+ N_{cp}(m+1)  +mK]\delta(m-\bar{m})\delta(k-\bar{k}) d\nu
\end{split}
\end{equation}

\subsection{OTFS}
Because \ac{OTFS} transmits successive \ac{CP}-\ac{OFDM} symbols, then for the $k$- symbol we get 
\begin{equation}
\DFT{M} \IndexM{\V{M}{N}{\ma{y}}}{:}{k}\approx  \tilde{\ma{h}}^{(e)}_k \odot \left[\DFT{M}\IndexM{\V{M}{N}{\ma{x}}}{:}{k}\right].
\end{equation}
Here,
\begin{equation}
\IndexV{\tilde{\ma{h}}_k^{(e)}}{q} = \frac{1}{M}\sum_{m=0}^{M-1} \tilde{h}(q,M_{cp}+m+k(M_o + N_{cp})).
\end{equation} 
Then by stacking the columns and using \eqref{eq:OFDM} , we get \eqref{eq:channel oTFS}.
\begin{equation}
\DFT{M_o}\V{M}{K}{\ma{y}} = \tilde{\ma{H}}^{(e)}\odot  \ma{X}^T + \tilde{\ma{Z}}, 
\end{equation}
where $\tilde{\ma{Z}}$ is the interference. 
\subsection{GFDM}
while one \ac{CP} per \ac{GFDM} is added then, 
\begin{equation}
\tilde{\ma{y}} = \tilde{\ma{h}}^{(e)}\odot  \tilde{\ma{x}} + \tilde{\ma{z}}.
\end{equation}
\begin{equation}
\IndexV{\tilde{\ma{h}}^{(e)}}{q} = \frac{1}{N}\sum_{n=0}^{N-1} \tilde{h}(q,N_{cp}+n).
\end{equation} 

\begin{itemize}
	\item[$C_1$.] Data precoding
	
	\item[$C_2$.] Windowing with window $\ma{W}_{K,M} \in \compl^{K\times M}$
	
\end{itemize}
The window depends on the type of modulator, thus 
\begin{equation}
\begin{array}{cc}
\ma{W}^{(\text{TD})}_{K,M} = K{\Z{M}{K}{\ma{g}}}^T &,  \ma{W}^{(\text{FD})}_{K,M} = K{\Z{K}{M}{\tilde{\ma{g}}}}
\end{array}
\end{equation}

In the time domain implementation, $\ma{X}_{K,M}$ contains frequency samples so, the time domain needs two further steps
\begin{itemize}
	\item[$T_3$.] Generating \ac{OFDM} symbols out of $\ma{X}_{K,M}$ 
	\begin{equation}
	{\V{M}{K}{\ma{x}}} = \frac{1}{M}\DFT{M}^H\ma{X}_{K,M}^T \label{eq:OFDM step}
	\end{equation}
	\item[$T_4$.] Time domain mapping
	\begin{equation}
	\ma{x} = \Vect{\left(\V{M}{K}{\ma{x}}\right)^T}. 
	\end{equation}
\end{itemize}

In the frequency domain implementation, $\ma{X}_{K,M}$ contains time domain samples so, we need 3 further steps
\begin{itemize}
	\item[$F_3$.] Generating \ac{SC} symbols 
	\begin{equation}
	{\V{K}{M}{\tilde{\ma{x}}}} = \DFT{K}\ma{X}_{K,M} \label{eq:OFDM}
	\end{equation}
	\item[$F_4$.] Frequency domain mapping 
	\begin{equation}
	\tilde{\ma{x}} = \Vect{\left(\V{K}{M}{\tilde{\ma{x}}}\right)^T}. 
	\end{equation}
	\item [$F_5$.] Time domain signal generation
	\begin{equation}
	\ma{x} = \frac{1}{N}\DFT{N}^H\tilde{\ma{x}}. 
	\end{equation}
\end{itemize}

\subsection{Unified implementation of demodulator}

The demodulator does the inverse operation. Thus, the first step is different and the remaining steps are the same. The type of the signal is specified by the equalizer output. Let $\ma{Y}_{K,M} \in \compl^{K\times M}$ be the preprocessed received signal, then

\begin{itemize}
	\item[$C_2$.] Windowing with receive window $\bar{\ma{W}}_{K,M} \in \compl^{K\times M}$
	\begin{equation}
	\hat{\ma{D}}_P = \bar{\ma{W}}_{K,M} \odot \ma{Y}_{K,M} 
	\end{equation}
	\item[$C_3$.] inverse of the precoding	
	\begin{equation}
	\hat{\ma{D}} = \frac{1}{M}\DFT{K}\hat{\ma{D}}_P\DFT{M}^H 
	\end{equation}	
\end{itemize}
The receive window depends on the type of demodulator 

In the time domain 
\begin{itemize}
	\item[$T_1$.] Convert the received signal to frequency domain 
	\begin{equation}
	\ma{Y}^{(\text{TD})}_{K,M} =  \left[\DFT{M}\V{M}{K}{{\ma{y}_{\text{eq}}}}\right]^T
	\end{equation}	
\end{itemize}
In the frequency domain 
\begin{itemize}
	\item[$F_1$.] Convert the received signal to frequency domain 
	\begin{equation}
	\ma{Y}^{{(\text{FD})}}_{K,M} =  \frac{1}{K}\DFT{K}^H\V{K}{M}{{\tilde{\ma{y}}_{\text{eq}}}}
	\end{equation}	
\end{itemize}

Based on this model the \ac{GFDM} modulation can be summarized in three steps as shown in in Fig.~\ref{fig:modulator}
\begin{itemize}
	\item[1.] Data precoding
	\begin{equation}
	\ma{D}_P = \frac{1}{K}\DFT{K}^H\ma{D}\DFT{M} 
	\end{equation}
	\item[2.] Windowing with window $K \Zbar{K}{M}{\tilde{\ma{g}}}$
	\begin{equation}
	\tilde{\ma{X}} = K \Zbar{K}{M}{\tilde{\ma{g}}} \odot \ma{D}_P
	\end{equation}
	
\end{itemize}

\begin{figure}[h]
	\centering
	\begin{subfigure}[b]{.8\linewidth}{%
			\includegraphics[width=1\linewidth]{figures/GFDM_modulator.eps}}
		\caption{Modulator}
		\label{fig:modulator}
	\end{subfigure}
	\begin{subfigure}[b]{.8\linewidth}{
			\includegraphics[width=1\linewidth]{figures/GFDM_demodulator.eps}}
		\caption{Deodulator}
		\label{fig:demodulator}
	\end{subfigure}
	\caption{GFDM modulator and demodulator. }	
\end{figure}
$\ma{A}$ can be expressed as \cite{nimr2017optimal}
\begin{align}
\Amat &= \frac{1}{M} \PI{M}{K}^T\U{K}{M}^H\La^{(g)}\U{K}{M}\PI{M}{K} \U{M}{K}^H, \label{eq: A-TD}
\end{align}
where 
\begin{equation}
\U{P}{Q} = \ma{I}_P\otimes\DFT{Q},\label{eq: U matrix}
\end{equation}
the receiver matrix can be expressed in the same model  
\begin{align}
\ma{B} &= \frac{1}{M} \PI{M}{K}^T\U{K}{M}^H\La^{(\gamma)}\U{K}{M}\PI{M}{K} \U{M}{K}^H, \label{eq: B-TD}
\end{align}
then 
\begin{equation}
\ma{B}^H\ma{A} = \frac{1}{M}\U{M}{K}\PI{M}{K}^T \U{K}{M}^H \La^{(\gamma)H}\La^{(g)}\U{K}{M}\PI{M}{K} \U{M}{K}^H
\end{equation}
For example to get \ac{ZF},
\begin{equation}
\La^{(\gamma)H} = \frac{1}{K}{\La^{(g)}}^{-1} = \ma{W}_t^{-1}
\end{equation}

With that we get
\begin{align}
\dft{\ma{A}}
&= \PI{M}{K}\U{M}{K}^H \La^{(\dft{g})}\U{M}{K}\PI{M}{K}^T \U{K}{M}\PI{M}{K}. \label{eq: A-FD}
\end{align}
where 
\begin{align}
\La^{(\dft{g})} &= \diag{\Vect{\Zbar{K}{M}{\dft{\mav{g}}}}}. \label{eq: D-FD}
\end{align}
then 
\begin{equation}
\tilde{\ma{B}}^H\tilde{\ma{A}} = K\U{K}{M}^H\PI{M}{K} \U{M}{K}^H \La^{(\tilde{\gamma})H}\La^{(\tilde{g})}\U{M}{K}\PI{M}{K}^T \U{K}{M}\PI{M}{K}
\end{equation}
\begin{equation}
\La^{(\tilde{\gamma})H} = \frac{1}{MK}{\La^{(\tilde{g})}}^{-1} = \ma{W}_t^{-1}
\end{equation}

\subsection{Received signal in dispersive channel}
Consider a \ac{LTV} channel, with the response response $H(l,n)$, following the derivation steps in the appendix, the received \ac{OTFS} signal after removing the \ac{CP} from each \ac{OFDM} symbol can be expressed as 
\begin{equation}
\DFT{M}\V{M}{N}{\ma{y}} = \tilde{\ma{H}}^{(e)}\odot  \ma{X}^T + {\ma{Z}} +\ma{V}, \label{eq:channel OTFS}
\end{equation}
where $\tilde{\ma{H}}^{(e)} \in \compl^{M\times K}$ is the equivalent channel defined by
\begin{equation}
\IndexM{\tilde{\ma{H}}^{(e)}}{p}{q} = \sum_{m=0}^{M-1}\sum_{l=0}^{M-1} H(l,N_{cp}+m+q(M + N_{cp}))e^{-j2\pi\frac{lp}{M}},
\end{equation}
$\V{M}{K}{\ma{y}}$ is the matrix after removing the \ac{CP}s, $\ma{Z}$ is interference terms results due to Doppler spread and $\ma{V}$ is the additive noise samples.
This allow the combination of the equalization within the demodulator.  
Namely, the receive window $\ma{W}_{\text{rx}}$ is computed based on the transmit window $\ma{W}_{\text{tx}}$ and the channel $\ma{H} ^{(e)}$. 
In a matrix representation  using\eqref{eq: Aotfs-TD}, we get
\begin{equation}
\begin{split}
\ma{y} &=\{\V{M}{K}{\ma{y}}\}^T\\
&=  \frac{1}{M}\PI{M}{K} \U{K}{M}^H\left[\ma{\Lambda}^{(h^{(e)})}\La^{(g)}\right]\U{K}{M}\PI{M}{K} \U{M}{K}^H \ma{d} +{\ma{v}}.
\end{split}
\end{equation}
Here, $\ma{\Lambda}^{(h^{(e)})} = \diag{\Vect{\tilde{\ma{H}}^{(e)}}}$ and $\ma{v}$ denotes the additive noise and interference. 
This matrix model is equivalent to a \ac{GFDM} signal  generated by a pulse shape $g^{(h)}$ that satisfies 
\begin{equation}
\ma{\Lambda}^{(h^{(e)})}\La^{(g)} = \diag{\Vect{\Z{M}{K}{g^{(h)}}}}.
\end{equation}
Therefore, we can generate a receive filter $\gamma^{(h)}$ which  also performs circular convolution on the receive signal. After equalization we get according to \ac{GFDM} circular receiver
\begin{equation}
d_{k,m} = \gamma^{(h)*}[-n]\circledast \left(y[n]e^{-j2\pi\frac{kn}{K}}\right)|_{n=mK}.
\end{equation} 
Due to this processing, the data symbols get equal \ac{SNR}, which is an important feature of \ac{OTFS}. On the other hand, the received \ac{GFDM}  after removing the \ac{CP} can be expressed as 
\begin{equation}
\tilde{\ma{y}} = \tilde{\ma{h}}^{(e)}\odot  \tilde{\ma{x}} + \tilde{\ma{z}} +\ma{v},\label{eq:channel GFDM}
\end{equation}
\begin{equation}
\mbox{ where }~ \IndexV{\tilde{\ma{h}}^{(e)}}{q} = \frac{1}{N}\sum_{n=0}^{N-1}\sum_{l=0}^{N-1} H(l,N_{cp}+n)e^{j2\pi\frac{lq}{N}}.
\end{equation} 
Therefore, additional channel equalization processing is required before the demodulator, Fig.~\ref{fig:otfs_demodulator}. 
As a result, the matrix model for \ac{GFDM}
\begin{equation}
\ma{y} = \ma{H}\ma{A}\ma{d}+\ma{v}. 
\end{equation}
Here,  $\ma{H} = \frac{1}{N}\DFT{N}^H\diag{\tilde{\ma{h}}^{(e)}}\DFT{M}$ is the circular channel matrix. In general, $\ma{H}\ma{A}$  does not have the \ac{GFDM} matrix structure. Therefore, the total equalization and demodulation is not circular and the data symbols at the output of the demodulator have different \ac{SNR}.

successively, i.e. $\ma{s} = \Vect{\DFT{M}^H\ma{X}_o^T}$, while in \ac{GFDM} the \ac{OFDM} symbols are permuted with the transpose, so that,   $\ma{x} =  \Vect{\ma{X}\DFT{M}^H}$.
Comparing the parameters, to generate \ac{OTFS} using the \ac{GFDM} modulator we use $M = M_o$, $K = N_o$, $\ma{W}_{\text{tx}} = K \Z{M}{K}{\ma{g}}$. In other words, the number of subcarriers in \ac{OTFS} becomes the number of subsymbols in \ac{GFDM} and vice versa. We can simply conclude the relation between both signals as in the form, 
\begin{equation}
\ma{s} = \PI{K}{M}\ma{x},
\end{equation}
where, $\PI{P}{Q}\in \Re^{PQ \times PQ}$ is the permutation matrix  that fulfills for any $Q\times P$ matrix~$\ma{X}$
\begin{equation}
\Vect{\ma{X}^T} = \PI{P}{Q} \Vect{\ma{X}},
\end{equation}
\begin{equation}
\U{P}{Q} = \ma{I}_P\otimes\DFT{Q},\label{eq: U matrix}
\end{equation}
where $\otimes$ is the Kronecker product. Moreover, by the vectorization of  \eqref{eq:x_gfdm}, the \ac{GFDM} modulation matrix $\ma{A}$ can be expressed as \cite{nimr2017optimal}
\begin{align}
\Amat &= \frac{1}{M} \PI{M}{K}^T\U{K}{M}^H\La^{(g)}\U{K}{M}\PI{M}{K} \U{M}{K}^H, \label{eq: A-TD}
\end{align}
\begin{align}
\mbox{with },~\La^{(g)} &= \diag{\Vect{\Z{M}{K}{\mav{g}}}}. \label{eq: D-TD}
\end{align}
As a result the \ac{OTFS} modulation matrix can be expressed as
\begin{equation}
\ma{A}_{\text{OTFS}} = \frac{1}{M} \U{K}{M}^H\La^{(g)}\U{K}{M}\PI{M}{K} \U{M}{K}^H. \label{eq: Aotfs-TD}.
\end{equation}
\begin{figure}[h]
	\centering
	\centering
	\begin{subfigure}[b]{.8\linewidth}{%
			\includegraphics[width=1\linewidth]{figures/OTFS_modulator.eps}}
		\caption{Modulator}
		\label{fig:otfs_modulator}
	\end{subfigure}
	\begin{subfigure}[b]{.8\linewidth}{
			\includegraphics[width=1\linewidth]{figures/OTFS_demodulator.eps}}
		\caption{Deodulator}
		\label{fig:otfs_demodulator}
	\end{subfigure}
	\caption{Unified GFDM and OTFS transceiver.}	
\end{figure}

%Then, we get 
%\begin{equation}
%\hat{\ma{D}}_P = \ma{D}_P + [\ma{W}_{\text
%	rx}- \ma{1}_{K,M}]\odot\ma{D}_P+ \ma{W}_{\text
%rx}\odot\ma{Z} + \ma{W}_{\text
%rx}\odot\ma{V}.
%\end{equation}
%The term $[\ma{W}_{\text
%	rx}- \ma{1}_{K,M}]\odot\ma{D}_P$ represents \ac{ISI}. If the data symbols $\ma{D}$ are uncorrelated, then  $\ma{D}_P$ is uncorrelated/ In the case of uncorrelated noise $\ma{V}$ and  
In a matrix representation  using\eqref{eq: Aotfs-TD}, we get
\begin{equation}
\begin{split}
\ma{y} &=\{\V{M}{K}{\ma{y}}\}^T\\
&=  \frac{1}{M}\PI{M}{K} \U{K}{M}^H\left[\ma{\Lambda}^{(h^{(e)})}\La^{(g)}\right]\U{K}{M}\PI{M}{K} \U{M}{K}^H \ma{d} +{\ma{v}}.
\end{split}
\end{equation}
Here, $\ma{\Lambda}^{(h^{(e)})} = \diag{\Vect{\tilde{\ma{H}}^{(e)}}}$ and $\ma{v}$ denotes the additive noise and interference. 
This matrix model is equivalent to a \ac{GFDM} signal  generated by a pulse shape $g^{(h)}$ that satisfies 
\begin{equation}
\ma{\Lambda}^{(h^{(e)})}\La^{(g)} = \diag{\Vect{\Z{M}{K}{g^{(h)}}}}.
\end{equation}
Therefore, we can generate a receive filter $\gamma^{(h)}$ which  also performs circular convolution on the receive signal. After equalization we get according to \ac{GFDM} circular receiver
\begin{equation}
d_{k,m} = \gamma^{(h)*}[-n]\circledast \left(y[n]e^{-j2\pi\frac{kn}{K}}\right)|_{n=mK}.
\end{equation} 
Due to this processing, the data symbols get equal \ac{SNR}, which is an important feature of \ac{OTFS}. On the other hand, the received \ac{GFDM}  after removing the \ac{CP} can be expressed as 
\begin{equation}
\tilde{\ma{y}} = \tilde{\ma{h}}^{(e)}\odot  \tilde{\ma{x}} + \tilde{\ma{z}} +\ma{v},\label{eq:channel GFDM}
\end{equation}
\begin{equation}
\mbox{ where }~ \IndexV{\tilde{\ma{h}}^{(e)}}{q} = \frac{1}{N}\sum_{n=0}^{N-1}\sum_{l=0}^{N-1} H(l,N_{cp}+n)e^{j2\pi\frac{lq}{N}}.
\end{equation} 
Therefore, additional channel equalization processing is required before the demodulator, Fig.~\ref{fig:otfs_demodulator}. 
As a result, the matrix model for \ac{GFDM}
\begin{equation}
\ma{y} = \ma{H}\ma{A}\ma{d}+\ma{v}. 
\end{equation}
Here,  $\ma{H} = \frac{1}{N}\DFT{N}^H\diag{\tilde{\ma{h}}^{(e)}}\DFT{M}$ is the circular channel matrix. In general, $\ma{H}\ma{A}$  does not have the \ac{GFDM} matrix structure. Therefore, the total equalization and demodulation is not circular and the data symbols at the output of the demodulator have different \ac{SNR}.

successively, i.e. $\ma{s} = \Vect{\DFT{M}^H\ma{X}_o^T}$, while in \ac{GFDM} the \ac{OFDM} symbols are permuted with the transpose, so that,   $\ma{x} =  \Vect{\ma{X}\DFT{M}^H}$.
Comparing the parameters, to generate \ac{OTFS} using the \ac{GFDM} modulator we use $M = M_o$, $K = N_o$, $\ma{W}_{\text{tx}} = K \Z{M}{K}{\ma{g}}$. In other words, the number of subcarriers in \ac{OTFS} becomes the number of subsymbols in \ac{GFDM} and vice versa. We can simply conclude the relation between both signals as in the form, 
\begin{equation}
\ma{s} = \PI{K}{M}\ma{x},
\end{equation}
where, $\PI{P}{Q}\in \Re^{PQ \times PQ}$ is the permutation matrix  that fulfills for any $Q\times P$ matrix~$\ma{X}$
\begin{equation}
\Vect{\ma{X}^T} = \PI{P}{Q} \Vect{\ma{X}},
\end{equation}
\begin{equation}
\U{P}{Q} = \ma{I}_P\otimes\DFT{Q},\label{eq: U matrix}
\end{equation}
where $\otimes$ is the Kronecker product. Moreover, by the vectorization of  \eqref{eq:x_gfdm}, the \ac{GFDM} modulation matrix $\ma{A}$ can be expressed as \cite{nimr2017optimal}
\begin{align}
\Amat &= \frac{1}{M} \PI{M}{K}^T\U{K}{M}^H\La^{(g)}\U{K}{M}\PI{M}{K} \U{M}{K}^H, \label{eq: A-TD}
\end{align}
\begin{align}
\mbox{with },~\La^{(g)} &= \diag{\Vect{\Z{M}{K}{\mav{g}}}}. \label{eq: D-TD}
\end{align}
As a result the \ac{OTFS} modulation matrix can be expressed as
\begin{equation}
\ma{A}_{\text{OTFS}} = \frac{1}{M} \U{K}{M}^H\La^{(g)}\U{K}{M}\PI{M}{K} \U{M}{K}^H. \label{eq: Aotfs-TD}.
\end{equation}
\begin{figure}[h]
	\centering
	\centering
	\begin{subfigure}[b]{.8\linewidth}{%
			\includegraphics[width=1\linewidth]{figures/OTFS_modulator.eps}}
		\caption{Modulator}
		\label{fig:otfs_modulator}
	\end{subfigure}
	\begin{subfigure}[b]{.8\linewidth}{
			\includegraphics[width=1\linewidth]{figures/OTFS_demodulator.eps}}
		\caption{Deodulator}
		\label{fig:otfs_demodulator}
	\end{subfigure}
	\caption{Unified GFDM and OTFS transceiver.}	
\end{figure}

\subsection{Properties of spreading}
Let 
\begin{equation}
\hat{\ma{D}}_P = {\ma{D}}_P + \ma{V},
\end{equation}
where $\ma{V}$ is the additive noise samples noise samples, then
\begin{equation}
\begin{split}
\hat{\ma{D}} &= \frac{1}{M}\DFT{K}\hat{\ma{D}}_P\DFT{M}^H = \ma{D} +   \underbrace{\frac{1}{M}\DFT{K}{\ma{V}}\DFT{M}^H}_{\bar{\ma{V}}}.
\end{split}
\end{equation}
Assuming that  the samples 
$\{v_{k,m} = \IndexM{\ma{V}}{k}{m}\}$,  are uncorrelated, i.e. 
\begin{equation}
\Ex{v_{k_1,m_1}v^*_{k_2,m_2}} = \sigma^2_{k_1,m_1}\delta_{k1,k2}\delta_{m_1,m_2},
\end{equation}
where $\delta_{x_1,x_2} = 1,~ x_1 = x_2$ and $0$ elsewhere. Therefore,  the noise samples $\bar{v}_{k,m} = \IndexM{\bar{\ma{V}}}{k}{m} $ have equal power
\begin{equation}
\Ex{|\bar{v}_{k,m}|^2} = \frac{1}{M^2}\sum_{m=0}^{M-1}\sum_{k=0}^{K-1}\sigma^2_{k,m}.
\end{equation}
The spreading is the essential part of the \ac{GFDM} processing.

\subsection{Conventional matrix representation}

In the conventional matrix representation, the \ac{GFDM} block can be expressed using a matrix $\ma{A}\in \compl^{N\times N}$ as 
\begin{equation}
\begin{split}
\ma{x} &= \ma{A}\ma{d},\\
\IndexM{\ma{A}}{n}{k+mK} &= g[<n-mK>_N]e^{j2\pi\frac{k}{K}n},
\end{split}
\end{equation}
where $\ma{d}= \Vect{\ma{D}}$ with $\IndexM{\ma{D}}{k}{m} = d_{k,m}$.
\noindent At the demodulator, a  matrix $\ma{B}\in \compl^{N\times N}$ is applied, such that
\begin{equation}
\begin{split}
\hat{\ma{d}} &=\ma{B}^H\ma{y},\\ \IndexM{\ma{B}}{n}{k+mK} &= \gamma[<n-mK>_N]e^{j2\pi\frac{k}{K}n}.
\end{split}
\end{equation}
Thus, the \ac{GFDM} demodulator and demodulator matrices follows the same structure, i.e. the columns are generated by circular shift in the time and the frequency domains of a prototype vector.

\subsection{Extended flexibility of GFDM }
In \ac{GFDM}, the main degrees of freedom includes the number of subcarriers $K$ and the number of subsymbols $M$. Both of them are exploited in the spreading step. Furthermore, the prototype pulse shape is another reconfigurable parameter, which is already represented in the windowing step. Further configuration can be exploited to extend the flexibility of \ac{GFDM} modem.
\begin{itemize}
	\item Flexible spreading: the spreading can be altered to enable or disable the spreading matrices.
	\item Flexible mapping:
	The conventional mapping preserves the spectral characteristics of the \ac{GFDM} signal. From mathematical point of view any permutation of the samples preserves the information, but leads to spreading of the spectrum. One practical case of the time domain mapping is to use the following mapping
	\begin{equation}
	\ma{x}_o = \Vect{\V{M}{K}{\ma{x}}}  =\frac{1}{M} \Vect{\DFT{M}^H\ma{X}^T}.
	\end{equation}
	This signal corresponds to $K$ sequential \ac{OFDM} symbols of length $M$.
	The mapping in the frequency domain can be exploited to perform \ac{FDMA}. The vector $\tilde{x}$ is divided into $U$ bands, each of length $N_u$ corresponds to a band allocated to the $u$-th user. This user generates a \ac{GFDM} block $\tilde{\ma{x}}_u$ of size $N_u$. In the mapping step the matrix ${\V{K}{M}{\tilde{\ma{x}}_u}}$ is mapped to $\ma{x}$ using the allocated indexes.
	\item  Flexible transformation: the \ac{DFT} or \ac{IDFT} transformation can be turned on or off in both domains to get more options. For example, in the frequency domain, we turn off the $K$-\ac{DFT} to get 
	\begin{equation}
	\ma{X} = {\V{K}{M}{\tilde{\ma{x}}}}.
	\end{equation}
\end{itemize}
This extended flexibility is exploited in the next section to generate \ac{OTFS} signal.

%One practical case of the time domain mapping is to use the following mapping
%\begin{equation}
%\ma{x}_o = \Vect{\V{M}{K}{\ma{x}}}  =\frac{1}{M} \Vect{\DFT{M}^H\ma{X}^T}.
%\end{equation}
%This signal corresponds to $K$ sequential \ac{OFDM} symbols of length $M$.
%The mapping in the frequency domain can be exploited to perform \ac{FDMA}. The vector $\tilde{x}$ is divided into $U$ bands, each of length $N_u$ corresponds to a band allocated to the $u$-th user. This user generate a \ac{GFDM} block $\tilde{\ma{x}}_u$ of size $N_u$. In the mapping step the matrix ${\V{K}{M}{\tilde{\ma{x}}_u}}$ is mapped to $\ma{x}$ using the allocated indexes.
%\item  Flexible transformation: the \ac{DFT} or \ac{IDFT} transformation can be turned on or off in both domains to get more options. For example, in the frequency domain, we turn off the $K$-\ac{DFT} to get 
%\begin{equation}
%{\V{K}{M}{\tilde{\ma{x}}_o}} = \ma{X}.
%\end{equation}
%\end{itemize}
